# Supplementary material for: Foundation Models For Seismic Data Processing: An Extensive Review
Source: arXiv:2503.24166 source file (2025-05-09)
Supplement: Supplementary file 1 [file appendix.tex]

\section{Appendix}

\subsection{Decoder}
\label{sec:appendix_decoder}

The current study concentrated on the architecture of the \ac{fm} used as an image encoder, while keeping the architecture and hyperparameters of the decoder constant across all experiments. Prior to this, we performed an initial investigation to determine the optimal architecture and hyperparameters for the demultiple task, as depicted in Figure \ref{fig:appendix_decoder}. This figure features two plots comparing the achieved \ac{psnr} with the number of decoder parameters. The left plot shows results using a \ac{swin} model as the encoder, while the right plot displays results with a \convnext{} model as the encoder.

The decoder architecture includes skip connections, the type of convolution block, and the up-sampling method. If skip connections are present, similar to the right side of a \unet{}, all four features extracted from the \ac{fm} are iteratively up-sampled and combined. Without skip connections, only the final feature is up-sampled and processed.
As seen in the figure, skip connections and the hierarchical features they enable are vital for achieving optimal results. While the performance gap is less significant with a \convnext{} as the encoder, there is still a difference of about 5 \si{\decibel}. When using a \ac{swin} model as the encoder, the gap widens to approximately 15 \si{\decibel}.
The choice of convolution block has a smaller impact on performance, but models with the newer \convnext{} blocks, as opposed to traditional double convolution blocks, consistently perform better with fewer parameters. This supports the performance difference observed in our studies between \efficientnet{} and \convnext{} models. The final architectural element examined was the up-sampling method. Generally, bilinear up-sampling seems to outperform transposed convolutions with fewer parameters.

After deciding to use skip connections, \convnext{} blocks, and bilinear up-sampling, the remaining hyperparameter is the bottleneck multiplier in the convolution block. Although increasing this improves performance, a multiplier of two was chosen to balance reduced performance and a simplified decoder. A smaller decoder places more emphasis on the encoder, the main focus of this study, and reduces training time, allowing for more experiments.

It is also noteworthy that the trends observed with a \ac{swin} model appear more linear, suggesting features that are more readily transferable.

\begin{figure}
  \centering
  \includegraphics[width=\textwidth]{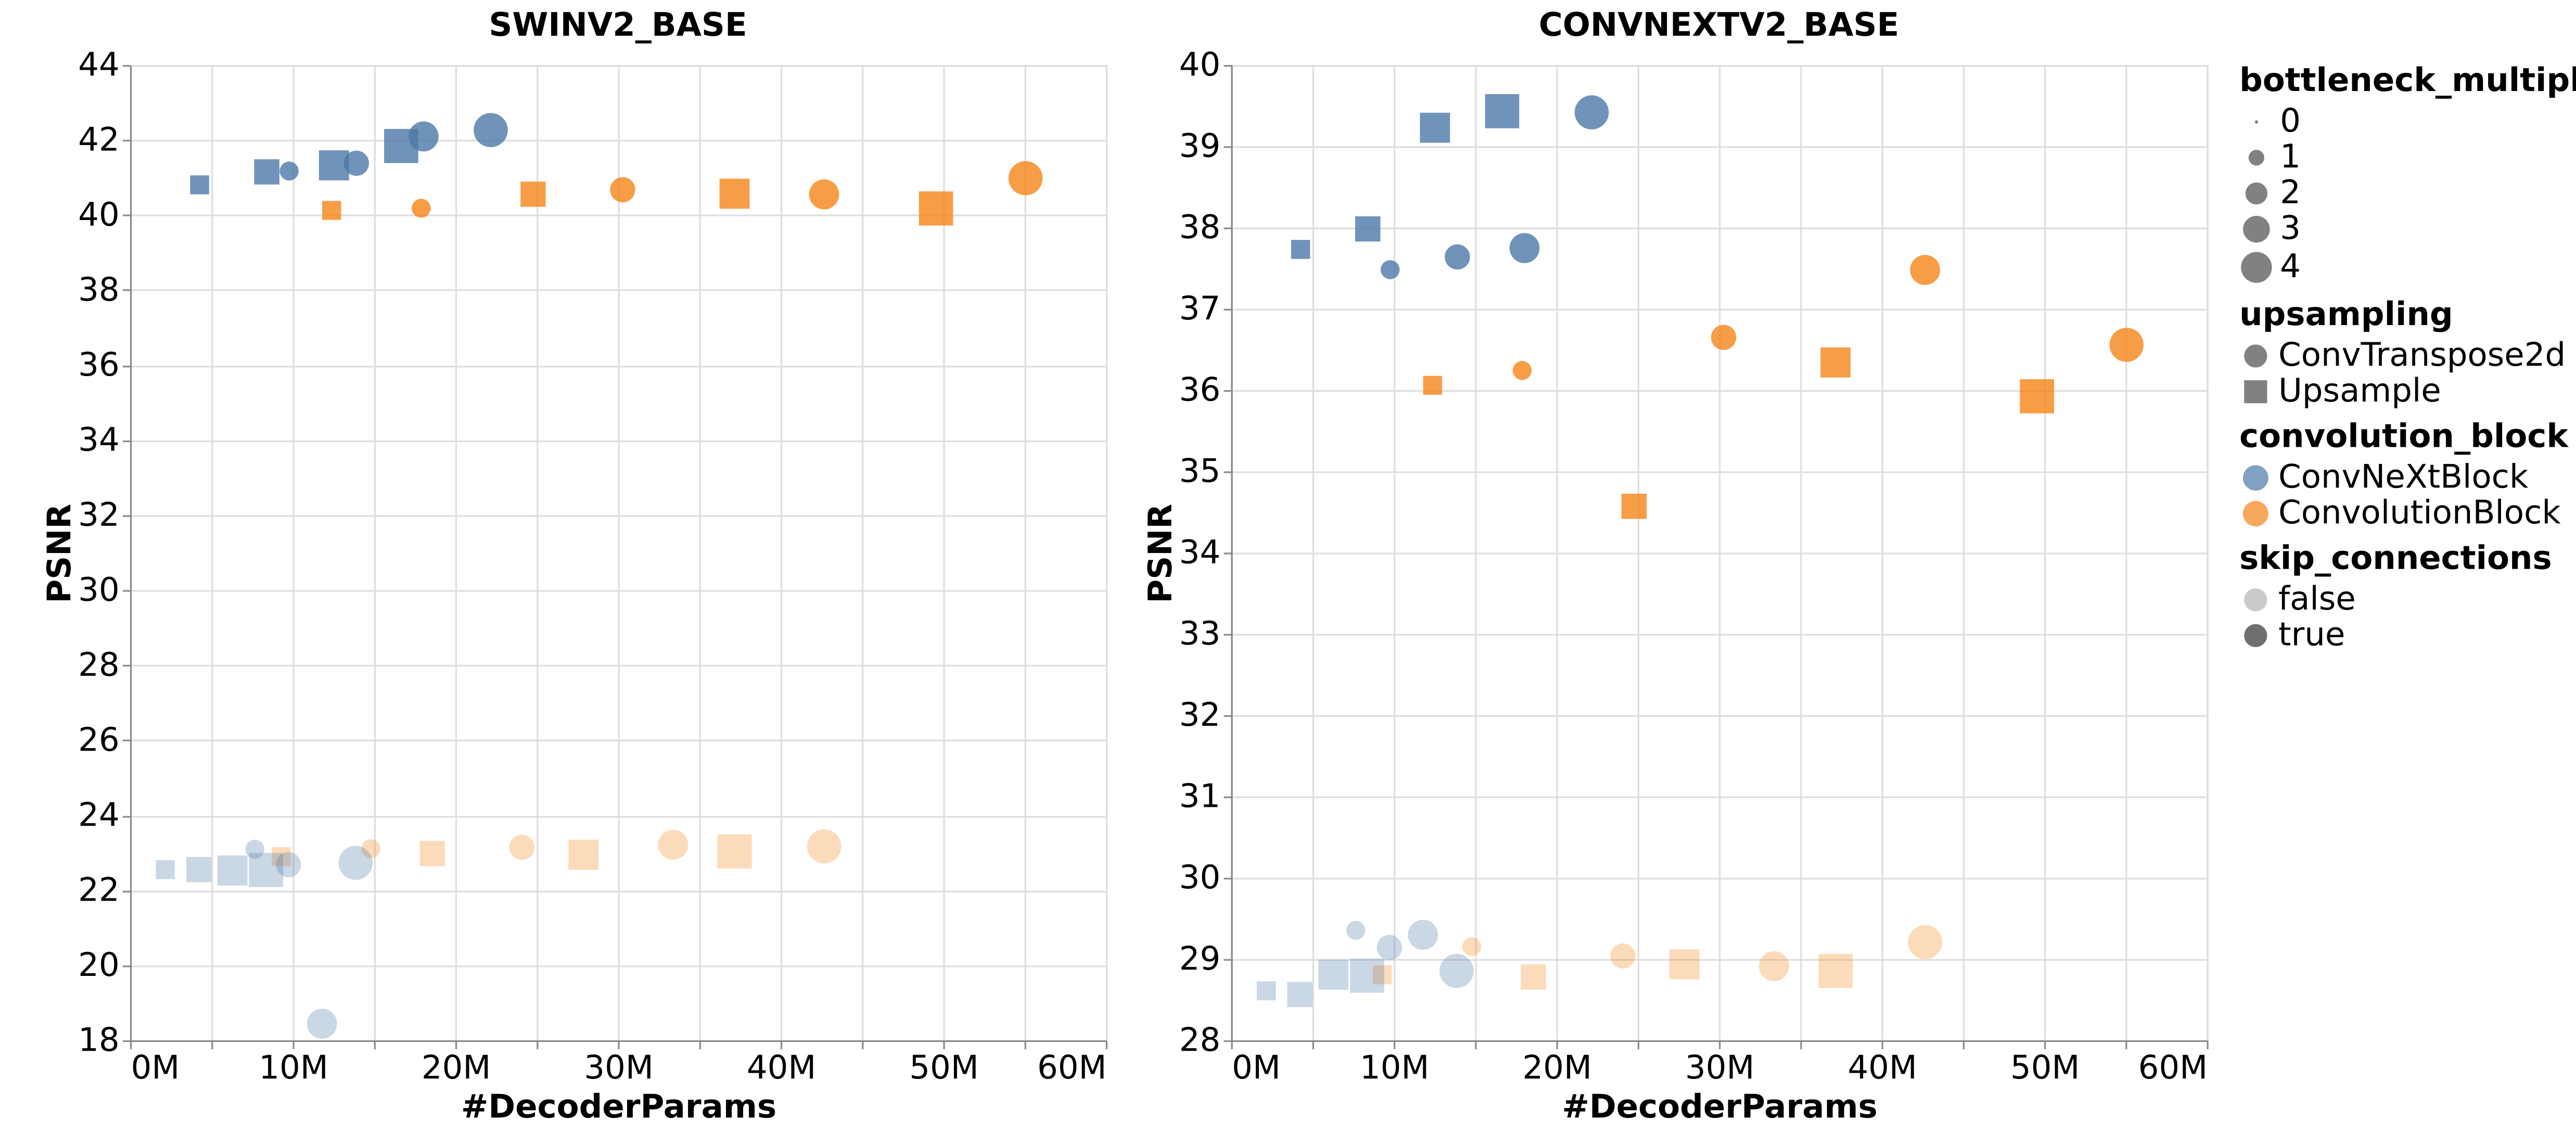}
  \caption{Hyperparameter analysis of the decoder.}
  \label{fig:appendix_decoder}
\end{figure}
